# Supplementary material for: Feature Purified Transformer With Cross-level Feature Guiding Decoder For Multi-class OOD and Anomaly Deteciton
Source: arXiv:2406.15396 source file (2024-04-30)
Supplement: Supplementary file 1 [file 12_appendix.tex]

\textbf{Appendix Section}
\section{Complexity Analysis of Image Compositions}
%\subsection{Comparative Complexity Assessment of Experimental Datasets }
%To further investigate the complexity across MVTec  and Mnist  dataset, we use tsne to visualize the encoder representation before MGM and APM as shown in Fig.\ref{}
%Supplementary material goes here.
\begin{table}[h]
\centering
\begin{tabular}{|l|l|l|l|}
\hline
            Dataset type        & MVTec & CIFAR10 & Mnist \\ \hline
Image Entropy value &    5.6   & 4.5     & 1.32  \\ \hline
\end{tabular}
\caption{The comparison table of the mean image entropy value for MVTec, CIFAR10, Mnist}
\label{tab:image_entropy}
\end{table}

In Sec. \ref{sec:topk}, we state that the complexity of the image compositions within the datasets significantly influences the optimal choice for \(k\).
Since the image entropy can be used to quantify and measure the information content, pixel distribution, randomness and structure of the image, we use it to estimate the complexity of the image compositions within the datasets.
It is calculated using the following steps:

\begin{enumerate}
  \item We calculate the histogram of the pixel values in the image. For a grayscale image with pixel values between 0 and 255, the histogram \( h \) has 256 entries, where each entry \( h(i) \) represents the number
 of pixels with the intensity \( i \).
  \item We normalize the histogram to obtain the probability distribution \( p \) of the intensity levels. To do this, each histogram number \( h(i) \) is divided by the total number of pixels \( N \) in the image:
  \[
  p(i) = \frac{h(i)}{N}
  \]
  where \( N = \sum_{i=0}^{255} h(i) \).
  \item Calculate the entropy \( H \) using the probability distribution:
  \[
  H = -\sum_{i=0}^{255} p(i) \log_2 p(i)
  \]
  where the sum is taken over all possible intensity levels, and \( \log_2 \) denotes the base-2 logarithm.
\end{enumerate}

Entropy \( H \) is a non-negative value that quantifies the average amount of information or uncertainty per pixel in the image. A higher entropy value indicates a more complex image with a greater variety of pixel values, while a lower entropy value suggests a simpler image with less variability in pixel values.

{\color{red}Table \ref{tab:image_entropy}} shows that the image entropy of MVTec and CIFAR10 is relatively higher than that of Mnist, which indicates that the image composition of Mnist is less complex than that of MVTec and CIFAR10.

\section{Statistical Modeling of Latent Space Boundaries in Relation to Dataset Variability}
\label{app:b}
\begin{table*}[]
\centering
\caption{The probability density value of the anomalous embedding from the multi-class PDF is on average higher than the single-class PDF, indicating that the model trained on multi-classes tends to generalize covariate anomalies.}
\resizebox{\textwidth}{!}{%
\begin{tabular}{|c|c|c|c|c|c|c|c|c|c|c|c|c|c|c|c|}
\hline
\multicolumn{16}{|c|}{Probability density value on MVTec} \\
\hline
& Tile & Leather & Bottle & Grid & Transistor & Wood & Screw & Hazelnut & Cable & Zipper & Metal nuts & Pill & Capsule & Carpet & \textbf{Mean} \\
\hline
Single-class & 0 & 0 & 0 & 0 & 0 & 0 & 0 & 0 & 0 & 0 & 0 & 0 & 0 & 0 & \textbf{0} \\
\hline
Multi-class & 3.1 & 1.0 & 1.4 & 4.3 & 2.3 & 4.5 & 2.5 & 5.4 & 9.6 & 5.9 & 8.0 & 1.0 & 5.8 & 3.3 & \textbf{4.1} \\
\hline
\end{tabular}%
}
\label{tab:MVTec_PDF_comparison}
\end{table*}

\begin{table*}[]
\setlength{\abovecaptionskip}{0pt}
\setlength{\belowcaptionskip}{0pt}
\caption{The probability density value of the anomalous embedding from the multi-class PDF is on average higher than the single-class PDF, suggesting that a multi-class based model tends to have a more general boundary for anomalous sampling in the latent space, especially for semantic anomalies.}
\begin{center}
\begin{tabular}{|c|cc|cc|cc|}
\hline
\multicolumn{7}{|c|}{\textbf{Probability density value on MVTec}} \\ \hline
\multicolumn{1}{|c|}{Class} & \multicolumn{2}{c|}{\{0,1,2,3,4\}} & \multicolumn{2}{c|}{\{1,3,5,7,9\}} & \multicolumn{2}{c|}{\{0,2,4,6,8\}} \\ \cline{2-7} 
& Mnist & CIFAR10 & Mnist & CIFAR10 & Mnist & CIFAR10 \\ \hline
Single-class& 0 & 0 & 0 & 0 & 0 & 0 \\ \hline
Multi-class & 2.3 & 2.1 & 2.5 & 3.2 & 2.8 & 2.9 \\ \hline
\end{tabular}
\label{tab:Mnist_CIFAR10_comparison}
\end{center}
\end{table*}

Each dataset has a unique statistical distribution that captures the variations and characteristics of its features. A reconstruction model is trained to capture this dataset and encode it in a latent space. This encoded latent representation is characterized by its own statistical properties, including a mean and variance that correspond to the distribution of the original dataset.
If the embeddings fall within this distribution in the latent space, they are considered to lie within a defined boundary — the region where the model expects the projections of the training data to lie.

As hypothesis shown in Sec. 3.2, the models trained on multi-class datasets exhibit more diverse latent representations due to the greater variability of the training data. This diversity broadens the distribution of the latent space, so that a wider range of embeddings may be considered normal. As a result, the likelihood that an anomalous embedding is within the boundary of normality of the latent space increases, potentially leading to lower sensitivity in detecting anomalies.

To substantiate this claim, we systematically conduct empirical experiments to substantiate this claim.
The experiment involves modeling the data embeddings of both single-class and multi-class settings from the datasets using a Gaussian mixture model (GMM). This allows us to estimate the Probability Density Functions (PDFs) that describe the likelihood that an anomalous embedding falls within the normal embedding distribution in the latent space:
\begin{itemize}
    \item \textbf{High probability density values:} The higher values of probability density for the anomaly sample indicate that anomalous embeddings are more likely to fall in regions of high PDF probability. This suggests that the model's valid boundary for the normal data embedding was shaped to encompass a wide range of variations, including those characteristic of anomalies.
    \item \textbf{Low probability density values:} Lower probability density values for an anomaly sample would indicate that the anomalous embeddings are more likely to fall in regions of low PDF probability. This suggests that the latent space of the model has a boundary that does not encompass a wide range of variation and is instead more closely tied to the characteristics of the normal data.
\end{itemize}

\subsection{Experimental setting}
The experiments were performed with the MVTec, CIFAR10 and MNIST datasets. For the single-class setting, the models were trained on data from one class only and the resulting embeddings were used to construct a Gaussian Mixture Model (GMM). The multi-class setting follows the procedures described in Sec. \ref{sec:experiment}.

To investigate whether training on a multi-class dataset increases the likelihood that covariate anomalies are captured by the valid latent space, we used embeddings of defective elements of a given class in the MVTec dataset as input to the GMM-derived probability density functions (PDFs). In terms of semantic anomalies, embeddings of classes that are considered anomalous (for example, if classes {0,1,2,3,4} are considered normal, then classes {5,6,7,8,9} are considered anomalous) were similarly tested against the estimated PDFs.

\subsection{Experiment result}
According to Table \ref{tab:MVTec_PDF_comparison}, the PDFs associated with the multi-class configuration for the MVTec dataset show a 4.9\% increase in density values attributed to anomalies compared to single-class models, indicating a more variant valid boundary in latnet space.

Moreover, Table \ref{tab:Mnist_CIFAR10_comparison} reflects that, in the Mnist and CIFAR10 datasets, single-class PDFs virtually eliminate anomalies, whereas multi-class PDFs assign significantly higher density values to these outliers, signaling an extension in the boundary's inclusivity.

\subsection{Conclusion}
Based on the above experimental result, we can statistically confirm the assertion made in Sec.\ref{sec:Discussion of the behavior of reconstruction network in multi-class dataset} that a reconstruction model trained on multiclass datasets inevitably leads to a more variant valid boundary that includes both the covariate and the semantic embedding.
\begin{table*}[]
\setlength{\abovecaptionskip}{0pt}
\setlength{\belowcaptionskip}{0pt} 
\caption{Evaluation of AUROC for three different settings (\{0,1,2,3,4\}, \{1,3,5,7,9\}, \{0,2,4,6,8\}) on CIFAR10 and Mnist}
\begin{center}
\begin{tabular}{|ccccccccccc|}
\hline
\multicolumn{11}{|c|}{\textbf{AUROC performence on Mnist and CIFAR10}}                                                                                                                    \\ \hline
\multicolumn{1}{|c|}{\multirow{2}{*}{}} & \multicolumn{2}{c|}{US \cite{bergmann2020uninformed}}   & \multicolumn{2}{c|}{FCDD+OE \cite{liznerski2020explainable}} & \multicolumn{2}{c|}{PANDA\cite{mishra2021vt}}          & \multicolumn{2}{c|}{MKD \cite{salehi2021multiresolution}}           & \multicolumn{2}{c|}{Ours} \\ \cline{2-11} 
\multicolumn{1}{|c|}{}                  & Mnist & \multicolumn{1}{c|}{CIFAR10}& Mnist & \multicolumn{1}{c|}{CIFAR10}& Mnist & \multicolumn{1}{c|}{CIFAR10} & Mnist & \multicolumn{1}{c|}{CIFAR10} & Mnist      & CIFAR10      \\ \hline
\multicolumn{1}{|c|}{\{0,1,2,3,4\}}     & 0.57 & \multicolumn{1}{c|}{0.54}& 0.65 & \multicolumn{1}{c|}{0.75} & 0.64 & \multicolumn{1}{c|}{0.68} & 0.69  & \multicolumn{1}{c|}{0.78} & \textbf{0.99} & \textbf{0.94} \\ \hline
\multicolumn{1}{|c|}{\{1,3,5,7,9\}}    & 0.55 & \multicolumn{1}{c|}{0.57}& 0.63 & \multicolumn{1}{c|}{0.79} & 0.59 & \multicolumn{1}{c|}{0.70} & 0.59 & \multicolumn{1}{c|}{0.70} & \textbf{0.86} & \textbf{0.91} \\ \hline
\multicolumn{1}{|c|}{\{0,2,4,6,8\}}    & 0.53 & \multicolumn{1}{c|}{0.54}& 0.64 & \multicolumn{1}{c|}{0.74} & 0.63 & \multicolumn{1}{c|}{0.78} & 0.55 & \multicolumn{1}{c|}{0.68} & \textbf{0.85} & \textbf{0.98} \\ \hline
\multicolumn{1}{|c|}{mean}               & 0.55 & \multicolumn{1}{c|}{0.55}& 0.64& \multicolumn{1}{c|}{0.78}& 0.62 & \multicolumn{1}{c|}{0.72} & 0.61 & \multicolumn{1}{c|}{0.72} & \textbf{0.90} & \textbf{0.94} \\ \hline
\end{tabular}
\label{tab:Mnist_comparison}
\end{center}
\end{table*}

\section{Comparisons to existing CNN-based algorithms }
As elucidated in Table \ref{tab:Mnist_comparison}, our approach markedly surpasses existing CNN-based algorithms in terms of AUROC performance on both the Mnist and CIFAR10 datasets. Notably, our algorithm demonstrates superior performance over the US \cite{bergmann2020uninformed}, FCDD+OE \cite{liznerski2020explainable}, PANDA \cite{mishra2021vt}, and MKD \cite{salehi2021multiresolution} models.

In the context of the Mnist dataset, our method achieves remarkable advancements, outstripping the US, FCDD+OE, PANDA, and MKD algorithms with average improvements of 35\%, 26\%, 28\%, and 29\% respectively across the \{0,1,2,3,4\}, \{1,3,5,7,9\}, and \{0,2,4,6,8\} settings.

In parallel, for the CIFAR10 dataset, our methodology consistently demonstrates a dominant performance. The mean AUROC scores for all evaluated settings exhibit substantial enhancements over the competing algorithms, exceeding the US, FCDD+OE, PANDA, and MKD by 39\%, 18\%, 22\%, and 22\% respectively.

These empirical results firmly position our method at the forefront in this domain, evidencing not just competitive, but in many cases, superior performance against the spectrum of existing algorithms in multi-class datasets. The uniform superiority across varied dataset configurations and settings underlines the robustness and adaptability of our approach, particularly in the realms of anomaly detection and image classification.
\section{The visualization of the data embedding from MAD-ProFP}
To verify that class-conditioned prototype serve as a anchor embedding in the latent space which guide the input embedding toward it in the latent space,
We use t-SNE \cite{van2008visualizing} to visualize the embedding of the abnormal data and normal data before/after our proposed module.\\
\textbf{Experimental setting}
In our experimental setup, we focus on class 8 (identified as the anomalous class) from the Cifar10 and Mnist datasets. Utilizing the class indicator results from the CTC, we select class 3 from Mnist and class 4 from CIFAR10 as the normal class data for comparative visualization. We extract two key embeddings: the encoder embedding (output from the transformer encoder) and the guided embedding (output from the MGM). These embeddings, alongside their respective class-conditioned prototype embeddings, are crucial for our analysis. Notably, each extracted embedding from the sample has a dimensionality of 196x256, where 196 represents the sequence length and 256 denotes the embedding dimension. \\
\textbf{Experimental result}
As depicted in Fig. \ref{fig:tsne}(a), in the Mnist dataset, we observe that the embeddings for both the anomalous class (class 8) and the normal class (class 3) are effectively guided towards the class 3 prototype embedding post-MGM intervention. Similarly, Fig. \ref{fig:tsne}(b) illustrates that in the CIFAR10 dataset, embeddings of the anomalous class (class 8) and the normal class (class 4) are also oriented near the class 4 prototype. These visualizations serve as empirical evidence, validating that the class-conditioned prototypes are instrumental in steering the embeddings towards a normality-aligned distribution within the latent space.

\begin{figure*}
\setlength{\abovecaptionskip}{0pt}
\setlength{\belowcaptionskip}{0pt} 
\centering 
\includegraphics[width=\linewidth]{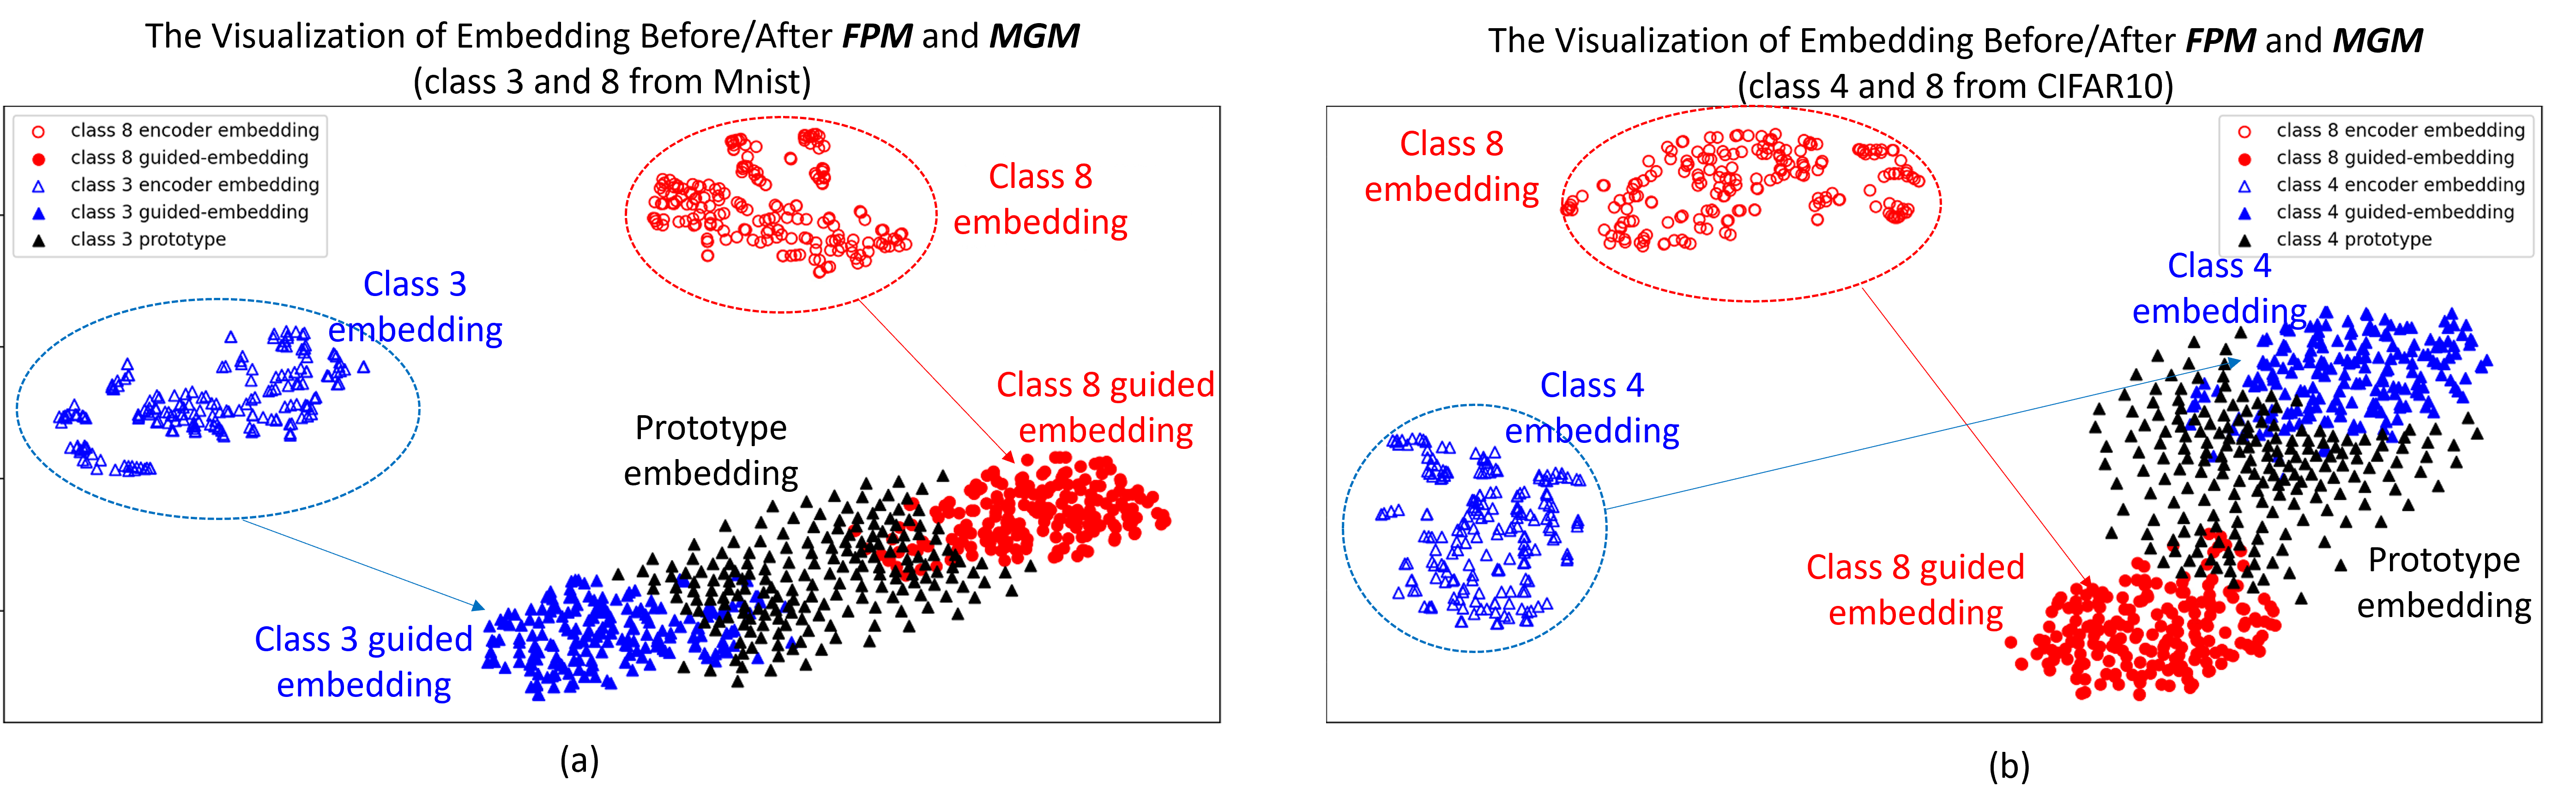}
   \caption{(a)The t-SNE \cite{van2008visualizing} visualization of embedding before/after FPM and MGM on Mnist dataset. The embeddings of anomalous (class 8) and normal sample (class 3) after FPM, MGM are guided toward class-conditioned prototype (class 3) ;
   (b)The t-SNE visualization of embedding before/after FPM and MGM on CIAFR10 dataset. The embeddings of anomalous (class 8) and normal sample (class 4) after FPM, MGM are guided toward class-conditioned prototype (class 4).}
\label{fig:tsne}
\end{figure*}
\section{The visualization of prototype embedddings in the prototype bank }
\textbf{Experimental setting}
To gain an intuitive understanding of the multi-class prototype embedding learned by our model, we visualize the prototype embeddings stored within the prototype bank, optimized using the MVTec dataset.
The visualization leverages a pre-trained deconvolution network, which is initially tasked with reconstructing refined feature maps, $x' \in \mathbb{R}^{H' \times W' \times C'}$, back into their original input images, $x \in \mathbb{R}^{H \times W \times C}$, prior to the CNN feature extraction process.

The prototype embeddings, $p^{i}_{\theta} \in \mathbb{R}^{s \times e}$, are reshaped into a dimensionality of $\mathbb{R}^{H' \times W' \times C'}$ to align with the deconvolution network's input requirements. This approach enables us to project the high-dimensional latent prototype embeddings back into the original input space, providing a visual interpretation of the semantic information encapsulated within these embeddings.\\
\textbf{Experimental result:}
Upon examining the visual outcomes depicted in Fig. \ref{vis_pro}, it becomes apparent that each prototype distinctly encapsulates the characteristic features of its respective class. It is observed that for categories with a higher degree of intra-class variability, such as variations in angle and color, the prototypes tend to represent these variations more abstractly. Examples of this include the prototypes for toothbrushes, screws, and metal nuts, which display a more abstract imagery in the visualization results, reflecting the greater variance in their training samples.

Conversely, classes characterized by more homogeneous features, such as bottles, pills, and tiles, result in visualizations that appear more cohesive and complete. It is important to note, however, that the abstract nature of a prototype's imaging does not necessarily indicate a lack of accurate encoding of the class data's normality. This is because the deconvolution network used for visualization is specifically trained to transform the CNN-extracted feature map $x'$ back into the original image.

From these visualization results, we can infer that our prototypes capture essential underlying features of class data. These features act as crucial guides for the normality in the reconstruction-based anomaly detection mechanism, reinforcing the effectiveness of this approach.
%We visualize each prototype embedding in the prototype bank trained with MVTec dataset as shown in Fig. \ref{}.
%Our design philosophy is to utilize prototype embeddings which encoded with underlying feature of the multi-class data to guide the reconstruction of anomaly data to induce a larger reconstruction error.
%We observed that the visualization result of each prototype repersent exhibit representative feature of the class data. prototype of toothbrush exhibit a more abstract presentation which the brush hair is composed of several color  since the training data include several color of toothbrush.
%As for class data which has less feature variant(angle, color), such as Bottle and Pill, the visualization result show a more 完整的影像呈現。 
%The above finding is also correspond to 

\begin{figure*}
\setlength{\abovecaptionskip}{0pt}
\setlength{\belowcaptionskip}{0pt} 
\centering 
\includegraphics[width=\linewidth]{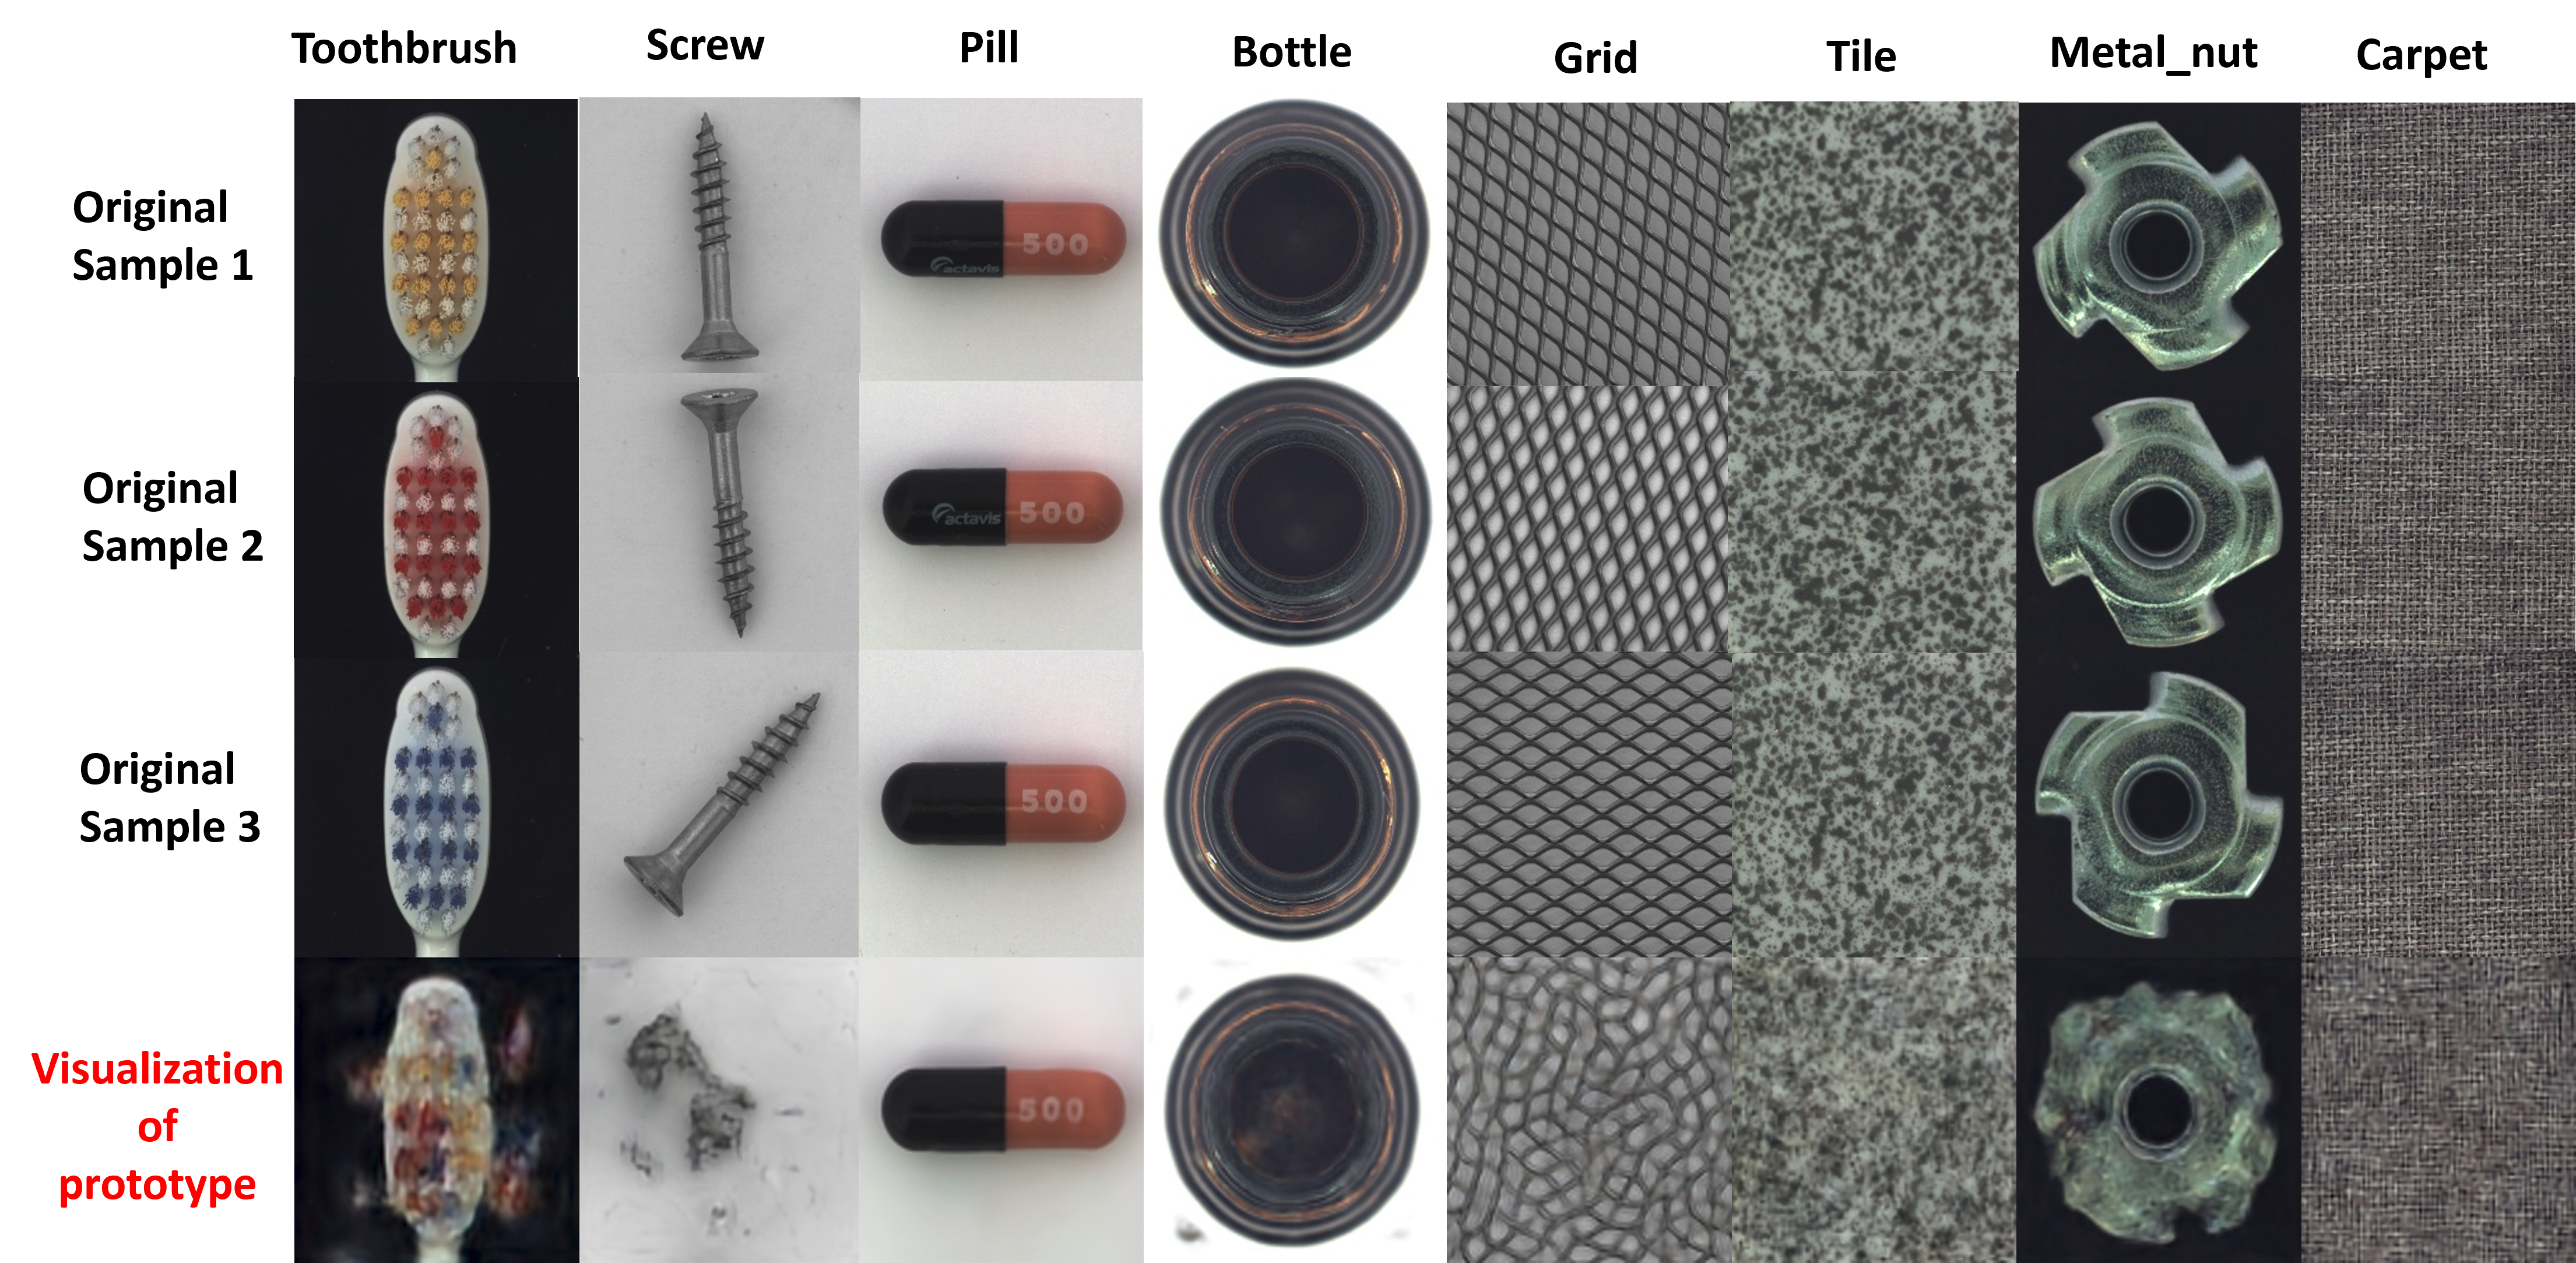}
   \caption{The visualization of Prototype Embeddings. The first three row displays samples of normal data from various classes in the MVTec dataset. The bottom row represents the visualizations of the corresponding prototype embeddings, reconstructed using a pre-trained deconvolution network. These visualizations provide insight into the characteristic features that the prototypes have captured for each class, serving as a reference for anomaly reconstruction within the MAD-ProFP framework}
\label{vis_pro}
\end{figure*}
